# Supplementary material for: Simple Visual Artifact Detection in Sora-Generated Videos
Source: arXiv:2504.21334 source file (2025-04-30)
Supplement: Supplementary file 1 [file appendix.tex]

\section{Appendix Section}
\label{sec:appendix_section}
Supplementary material goes here.
